# Supplementary material for: Segmentation in Style: Unsupervised Semantic Image Segmentation with Stylegan and CLIP
Source: arXiv:2107.12518 source file (2021-11-18)
Supplement: Supplementary file 1 [file X_supplementary.tex]

\appendix

% --- PDF will be split by an editor (e.g. macOS preview), so need to restart from page 1
\setcounter{page}{1}

% --- repeat the title (AT: haven't found a more elegant way to do this...)
\twocolumn[
\centering
\Large
\textbf{[CVPR2022] Official LaTeX Template} \\
\vspace{0.5em}Supplementary Material \\
\vspace{1.0em}
] %< twocolumn
\appendix

\section{Extra experiments}
\lorem{2}

\section{Dataset description}
\lorem{2}

\section{Qualitative results}
\lorem{2}
